# Supplementary material for: Learning Language Games through Interaction
Source: arXiv:1606.02447 source file (2016-06-08)
Supplement: Supplementary file 1 [file appendix.tex]

\section{Appendix}
We provide some plots, examples, and transcripts that did not make to
the main paper.

\subsection{More examples for pragmatics}
\begin{table}
\begin{tabular}{ c | r r r r } 
& $z_{\logf{rm r}}$ & $z_{\logf{add c}}$ & $z_{\logf{rm c}}$ & $z_{\logf{add r}}$ \\ \hline
& \multicolumn{4}{c}{$\listen{0}(z|x)$} \\
 \hline
 $\utt{remove red}$   & 0.5 & 0.1 & 0.2 & 0.2 \\ 
 $\utt{add cyan}$       & 0.1 & 0.5 & 0.2 & 0.2\\ \hdashline
 $\utt{remove cyan}$ & 0.4 & 0.4 & 0.2 & 0.2\\ 
(\# features) & 3 & 3 &  2 & 2\\ \hline
& \multicolumn{4}{c}{$\speak{1}(x|z)$} \\
 \hline
$\utt{remove red}$    & 0.6 & 0.1 & 0.33 & 0.33\\
 $\utt{add cyan}$       & 0.1 & 0.6 & 0.33 & 0.33\\ \hdashline
 $\utt{remove cyan}$ & 0.3 & 0.3 & 0.33 & 0.33\\ \hline
& \multicolumn{4}{c}{$\listen{1}(z|x)$ ommited}
\end{tabular}
\caption{example how pragmantic inference is useful for the kind of generalization we want. Suppose our features are unigrams in utterances matched with unigrams and bigrams of the predicates on the formulas, then this table is realistic.}
\label{tab:example2p}
\end{table}

\begin{table}
\begin{tabular}{ c | r r r r } 
& $z_{\logf{rm r}}$ & $z_{\logf{add c}}$ & $z_{\logf{rm c}}$ & $z_{\logf{add r}}$ \\ \hline
& \multicolumn{4}{c}{score = \# features $\times \eta$} \\
\hline
$\utt{remove red}$   & 6 $\eta$ & 0$\eta$ & 1$\eta$ & 1$\eta$ \\
$\utt{add cyan}$       & 0 $\eta$ & 6$\eta$ & 1$\eta$ & 1$\eta$\\ \hdashline
$\utt{remove cyan}$ & 3 $\eta$ & 3$\eta$ & 2$\eta$ & 2$\eta$\\ \hline
& \multicolumn{4}{c}{$\listen{0}(z|x) \propto \exp(s)$} \\
\hline
$\utt{remove red}$   & 0.74 & 0.06 & 0.10 & 0.10 \\
$\utt{add cyan}$       & 0.06 & 0.74 & 0.10 & 0.10\\ \hdashline
$\utt{remove cyan}$ & 0.3 & 0.3 & 0.2 & 0.2\\ \hline
& \multicolumn{4}{c}{$\speak{1}(x|z)$} \\
\hline
$\utt{remove red}$   & 0.67 & 0.06 & 0.25 & 0.25 \\
$\utt{add cyan}$       & 0.06 & 0.67 & 0.25 & 0.25\\ \hdashline
$\utt{remove cyan}$ & 0.27 & 0.27 & 0.5 & 0.5\\ 
\end{tabular}
\caption{The computer saw the two examples above the dashed line,
and did a batch update with a learning rate of $\eta=\log(3/2)$, and for simplicity we used
$p(z|x;\theta=0)\approx 0$. 
The features used are unigrams in the utterance matched with unigrams
and bigrams of predicates. So we get 6 features with non-zero weights for $u=\utt{remove}, \utt{red}$, we get $u$\means\logf{Red},
$u$ \means\logf{remove}, and
\mbox{$u$ \means\logf{remove}$,1,\logf{Red}.$} {\bf top}: the score for each
utterance after the first update, {\bf mid}: probabilities assigned by
the literal listener $\listen{0}(z|x)$,  {\bf bot}: the pragmatic speaker.}
\label{tab:example2}
\end{table}

\begin{figure}[ht]
\begin{center} 
\includegraphics[width=0.4\textwidth]{plots/pragbetterworse.pdf}
\end{center}
\caption{\label{fig:pragbetterworse} each dot is a player, the x-axis is the
  proportion of examples by this player where the baseline ranks the
  correct action higher or equal. y-axis: the pragmatics listener ranks the
  correct action higher or equal. All together, pragmatics performed
  worse for only 17 out of 98 player in terms of ranking position.} 
\end{figure}

\subsection{Data analysis}
{\it
\begin{itemize}[noitemsep]
\item This is SO SO cool. I wish there were a way I could better contribute
because this research seems to be just insanely interesting and
worthwhile.

\item That was probably the most fun thing I have ever done on mTurk. I look
forward to more things like this! Thanks!

\item Wow this was one mind bending games. My score was 73.8, but maybe I could get a little
better score if I had more time. I will be waiting for its next
version.

\item That was very fun, please email me if you have any other hits like
this in the future :)

\item This HIT was interesting and fun. At first I thought the directions were confusing and then I started working and I got really good at it. Hope to do more like this!
\end{itemize}
}

\begin{figure}[ht!]
\centering
\mbox{\includegraphics[height=1.9in]{plots/tokentypes.pdf}
  \includegraphics[height=1.9in,trim={0.7cm 0 0 0},clip]{plots/tokencounts.pdf}}
\caption{the number of scrolls needed by token types and token counts.}
\label{fig:scrollvstokens}
\TODO{consider cutting, or appendixing}
\end{figure}
More quantitatively, we consider the number of token types used, and
the average number of tokens per utterance. They are somewhat predictive of the game
performance as measured by number of scrolls. \reffig{scrollvstokens}
shows a very noisy picture of this. We find that players who used
20-40 different token types, and who use utterances of 3-6 tokens long tend to perform better. 
This number of token types is comparable to the 12 predicates in \reftab{grammar} if we
account for functional words and plural forms.
